# Supplementary material for: Exploiting Physical Dynamics to Detect Actuator and Sensor Attacks in Mobile Robots
Source: arXiv:1708.01834 source file (2017-08-06)
Supplement: Supplementary file 1 [file supplementary.tex]

\section{Supplementary Material}
\subsection{Previous Submission Reviews}
\textbf{Submission}: \emph{IEEE Symposium on Security and Privacy, SP 2017, San Jose, CA, USA}

\textbf{Reviewer 1}\\
Overall merit

\textbf{3. Weak reject}\\
Strengths

cool/emerging problem with potential applications to autonomous deployments in the future\\
Comments

This seems a new and exciting problem domain but the current paper seems to have several shortcomings:

1.  Lack of clarity in core algorithm description:

Even after multiple reads I was unable to wrap my head around the basic algorithm design -- The pseudocode boxes  in Algo 1 and Algo 2 are practically undecipherable. I didnt even understand what type of anomaly detection the approach was using here -- timeseries vs MDP vs HMM

2. Narrow scope

The paper seems to start with a grander vision of autonomous robots/autonomous driving but the actual algo and design seems to be much narrower. For instance this exhaustive search over $2^m$ combinations where m is the number of sensors cant possibly work in an actual car setting since the number of sensors can be in the high thousands! I would scope the paper better

3. Weak evaluation

The evaluation seems to be quite toy and not really stressing the core design in any meaningful way vs adversarial evasion

4. The "insight" may be overfitting?

The main insight is this correlation. But I cant help wonder if this is somehow overfitting to the very specific set of toy robots you use. How robust is this to adversarial evasion? how general is this insight across other classes of robots and robotic applications? This may be true but as of now its speculative and oversold

Other minor comments:
-- these autonomous car/GPS attacks are orthogonal to your problem -- needless oversell

-- what is nonlinear? what about nonlinearity makes the problem hard?

-- it seems that noise and adversarial injection of sensor are the same type of problem. in any case its not clear what in the design actually handles either

-- how is this RIDS different from any other anomaly detection system or estimation based system? it seems like a standard estimation-detection problem?

-- why is CAN etc relevant to your paper?

-- it is really hard to get any insight or intuition on the core idea of this correlation. why should we believe this is generalizable?

-- eval is structured poorly as a data dump -- focus on 1-2 core results rather than do a data dump

\textbf{Reviewer 2}\\
Overall merit

\textbf{3. Weak reject}\\
Strengths

The problem addressed by this paper is interesting, and will be increasingly important as CPS become more ubiquitous.

The proposed approach does not make any specific trust assumptions about the sensors in a system, but only that some of them aren't compromised.

The approach is applied to a physical robot (not just simulated), and evaluated under several attack scenarios.\\
Comments

This paper covers an interesting topic, and gives a fairly extensive evaluation of a sensor/actuator attack detection system under an impressive number of attack scenarios. Perhaps the most interesting idea in this work is that of using sensor redundancy and hypothesis testing to estimate not just which parts of the system are under attack, but also detailed information about the properties and extent of the attack. This purportedly allows the approach to function without having to make static trust assumptions about any of the sensors, which would seem to make the work relevant for realistic setting, where such requirements may be infeasible.

While the paper is heavy on notation, and Algorithms 1 and 2 appear to give quite a bit of implementation detail, it seems that it is overall light on details that would justify the security of the approach, and quantify its limitations. Near the beginning, the authors assert that as long as not all of the sensors are compromised, the detection system will work. It isn't clear where this (very important) point is demonstrated anywhere in the paper.

Additionally, this claim runs contrary to one's intuition. Supposing the robot had two geolocation sensors, if one were compromised for the full duration of an execution, and presented consistent readings there were somehow skewed (perhaps translated by a fixed amount), how could the "mode selector" conclude that one mode is more likely than the other? To do so, the system would need to encode some prior assumptions, which would make much of what this system accomplishes unnecessary. To show that this approach works under the threat model outlined 2B, the paper should give a rigorous argument that the correct mode will always be selected (if it exists).

\textbf{Reviewer 3}\\
Overall merit

\textbf{4. Weak accept}\\
Strengths

This is a cool problem.
The algorithm seems solid.
They evaluate it on a real platform and even demonstrate a robot
  successfully completing its mission in the presence of attack,
  whereas it could not complete the mission without their system.\\
Comments

The writing could be improved.  There's lots of typos and grammatical
errors.  I think this work deserves a good presentation.

One major question is whether this is a security paper.  I think this
algorithm is really more appropriate for detecting malfunctioning
sensors rather than sensors under attack.  For example, it seems this
algorithm could have prevented the crash of Birgenair flight 301, which crashed
due to a nest insects had built in one of its Pito tubes.  Pito tubes
are used to measure airspeed, and the aircraft had 3 of them, but the
pilots relied only on the broken one.  If the aircraft had been
equipped with the system in this paper, I bet it would have flagged
that sensor as aberrant and alerted the pilots.

But adversarial failures are very different.  An adversary will make
your sensors or actuators fail in the worst possible way.  And I don't
think this paper really evaluated any well-crafted attacks on the
sensors or actuators in their robot.

But this is the first paper to really push in this direction, so I'm
willing to let that pass.  I think it's exciting to imagine the
follow-on work this paper could potentially inspire.

I wonder if it is possible to improve the efficiency of the
brute-force search over all possible subsets of sensors.  I think this
will be important because I doubt future robots will have only a few
sensors.  I bet they'll have a lot, e.g. > 100.  For example, if the
robot has n sensors, then we can pick a random starting subset of k
sensors and run their brute-force algorithm to obtain a subset k' of
sensors that appear to all be consistent with each-other.  We can then
add other sensors to this group one by one to find the largest set of
sensors that are consistent with the original group of k' sensors.  We
then repeat the process on all the remaining sensors, eventually
partitioning the set of sensors into groups, where all the sensors in
each group are consistent with each-other.  If we end up with all
sensors in a single group, then there is no attack.  Otherwise, we can
select the largest group as the authoritative group.

I also read the prior reviews, and the authors have done a significant
amount of work to improve the paper and the underlying research (and
experiments) based on the past feedback, so I think this paper
deserves fresh from-scratch reviews.

\textbf{Reviewer 4}\\
Overall merit

\textbf{2. Reject}\\
Strengths

Interesting goal, robot security is a growing concern and well motivated
Experimental study with realistic robotics testbed.\\
Comments

- The high level idea is fairly straightforward, so the strength of this paper should rest on the execution or difficult problems solved. The algorithm and nonlinear robotics model is straightforward.

The main problem is the attack model is fairly simplistic. What are the attackers’ goals? Just to cause a mission failure / a collision? The attack vectors here are, quite literally, vectors of perturbation applied to one or more sensors or actuators. This paper would be most improved by evidence showing that deployed robotics systems are vulnerable to the attacks targeting particular sensors of the kind modeled here, or that actual attacks use mechanisms like this.

        Could an attacker playing against this detection system find a way to cause the maximum amount of harm, while evading detection?

- Is there any inherent difference between an attack and an ordinary failures? The same mechanisms used here has also been used in fault tolerance. The paper would be more interesting if there was some explanation of why active attacks require special treatment or pose additional difficult problems that need technical solution.

- The main weaknesses are that the attack scenario is not that convincing and fairly weak. Attacks that involve too many sensors or actuators will not be detectable or recoverable. “Admittedly, such attacks could be possible, however, it is extremely difficult to launch such attacks.” Not much evidence is provided for this though.

\textbf{Submission}: \emph{26th USENIX Security Symposium, USENIX Security 17, Vancouver, BC}

\textbf{Reviewer 1}\\
Overall merit

\textbf{3. Weak accept}\\
Strengths

Interesting approach applied to mobile robots\\
Comments

Threat model need to be verified

Security Analysis should be improved

Security detection model is not very novel

The paper is well-written and well-executed. The idea to embed an intrusion detection system inside a mobile robot is really interesting and open a lot of interesting research questions, not only on the design of the defensive mechanism but also on the impact of the attack. In this direction the authors implemented several interesting attack scenario on real mobile robot where they show a potential impact on the mobile robot abilities.

However, I have some concerns about this paper. For example the authors chose a Threat model where they said the attacker can compromise only a part of the sensors but not all of them. They said that to the best of the their's knowledge no reported attack is launched being capable to compromise all the sensors. In the software architecture described in the paper each sensors is associated to a piece of code and then we have the planner code that is taking input from all the sensors and make the final decision. It would be great to understand details about real software architecture, planner and sensors' firmware, in terms of size, programming language, security mechanisms in place and potential attack points. In this way, we can better evaluate the TCB of the entire architecture.

The core of the detection algorithm is based on a prediction algorithm that is able to find out some discrepancy among several sensors behavior. The authors discuss in section 5.7 the evasive attacks, it would be great if they can discuss more in details about a possible mimicry attack that can base its own efficacy on the noise produced by the sensors. An attacker can take advantage of this noise area and perform a successfully mimicry attack.

In order to judge the novelty of the detection algorithm, it would be great if the authors can compare their method with the state of the art of the detection techniques used for mobile robots and show the strength and weaknesses of the proposed method.

\textbf{Reviewer 2}\\
Overall merit

\textbf{2. Weak reject}\\
Comments

The authors start by presenting the reference architecture,
with independent sensing and actuation workflows, and assume
that each of them can be compromised - either with a software
attack, a signal interference, or even a physical damage. I
found this (threat|robot) model very clear and able to capture
well different types of attacks on complex systems-of-systems
architectures. My only negative comment about the threat model
is the fact that the authors assume that when a workflow is
compromised, this gives the attacker any advantage to also
exploit the rest of the system. In particular, I believe that
if one workflow is compromised, it is reasonable to believe the
attacker can use it as a stepping stone to attack the planner.

I am also not sure that the planner is much simpler (in term
of code) than the sensing and actuation workflows. Actually,
in some cases I would expect quite the opposite.

Regarding the multi-mode solution, I do not understand why
there is only one mode per sensor, and not one for each
combination of trusted and untrusted sensors instead. Is it to
minimize the required resources? Is it because the remaining
combinations would not provide any benefit? Some experiments
would help to better understand this point.

Also, it is not clear how the likelihood of each mode is
computed. In particular, I really cannot understand how the
system can not only identify that an attack is ongoing, but it
can also reliably determine which sensors are under attack. For
instance, let's take the Khepera experiment. If the attacker
alters both the LiDar and the IPS to report no motion, but the
wheel sensor reports some motion .. two things are possible:
either the wheel is under attack and it is faking some
measurement, or the other two sensors are under attack and
report no values. How can the system distinguish between the
two cases? Would it just assume that the first case is more
likely than the second? So, the system always assume the
easiest attack condition to explain the current values?

RIDS uses the kinematic and sensor functions as well as all
the readings to estimate the robot state using multiple
parallel models. This seems comparatively more complex than the
original task running in the planner.. thus making RIDS a
relevant burden from a computational point of view.
It would be interesting to know what kind of computational
requirements it imposes to the robot and understand if this
is feasible without incurring in additional costs.

Another point that deserves some discussion is how
representative is the robot used in the experiment. A test on a
robot with three position sensors seems like the optimal case
for the presented technique (not too many, but plenty of
redundancy). What about much more complex systems - such as a
car, where there are hundreds of independent ECUs? I am not
saying that the authors should be able to test on a car (of
course it would be fantastic) but at least it would be good to
discuss how more complex cases could be addressed. Also,
not all sensors have a sibling that provides redundant information
for cross-checking the state. This may be common for position
sensors, but is this the only type of sensor that is protected
by this approach? What about a temperature sensor?

To conclude, I found the presented technique interesting but
it seemed too limited in its scope (only position-related attacks
on mobile robots) and in the type of attacks it can detect
(a compromised actuator that all in a sudden steers the robot
down a cliff or stops a car in the middle of a highway
would not be detected in time by this technique).

\textbf{Reviewer 3}\\
Overall merit

\textbf{2. Weak reject}\\
Strengths

Important area, and one that is worth greater attention.

The system appears to work for the scenarios presented.\\
Weaknesses

The system seems to work in a very limited setting using expected
  techniques.

There is no insight into how sensors should be picked, yet alone
  balanced.

There are significant presentation issues.

This is an important area, and one worth more attention. I particularly
appreciated that the authors took the time to build their techniques and
test them. For the tests performed, the authors do a convincing job of
demonstrating that their proposed techniques indeed have value.

There are a number of concerns that I have about the work in its current
form. The first is that the testing environment is very artificial. The
mobile robots are constrained to a 3x3 space, with no real obstacles or
imperfections (e.g., sand, dirt, uneven surfaces). That makes the
results here seem absolutely best case - slow moving robots in a
protected space. Accordingly, it was difficult for me to believe that
the false positive rates seen here were representative of what devices
would see in the real world. Granted, I appreciate that mobile robots
encompass a potentially huge range of devices and conditions, but the
selected platform did not give me greater confidence. For instance, if
you had picked something like a Roomba, which arguable works in a
similarly constrained environment, would the same set of sensors be
available?

The approach here makes a lot of sense - compare a suspected good state
to the current state and then determine whether or not you are outside
of some envelope of expected behavior. What was missing was the insight
here. For instance, how much energy is required to implement this
approach, and how does it impact the overall lifetime of the device?
Additionally, how should someone building a mobile robot platform pick
the sensors they are using? Must they guarantee that at least three
overlap? Is this realistic on many platforms? This is where the work
could really excel.

As the last major point, the work has significant presentation issues.
The authors should go back through and improve the flow of the text.
Additionally, it is unclear what the reader should get from Figure 6 -
the fonts are tiny, and it is never stated what we should look for or
understand.

\textbf{Reviewer 4}\\
Overall merit

\textbf{4. Accept}\\
Comments

This is an interesting paper on an important topic. The high-level ideas are
expressed clearly.

If I understand correctly, this technique should work for any robot that has
multiple sensors from which the entire robot state can be estimated. You give
an example of a situation where it doesn't work in section 6. It would be nice
if you could expand on the specifics of what RIDS requires and what its
limitations are. I would imagine that there are a number of robots whose
complete state can only be computed from all of its sensors. In other words,
cases where a particular sensor is essential because no other (group of)
sensor(s) duplicates its functionality. In that case, is there anything that
RIDS can do?

In the introduction, you give steering wheels and accelerators (gas pedals) as
examples of actuators. These didn't seem like great examples to me. The
accelerator no longer connects directly to the car's throttle. It's just a
sensor that is read by the engine control module. The steering wheel does
have a physical linkage to the front wheels but I don't think I'd call it an
actuator. It's connected to a hydraulic actuator. (Actually, I think it's
pretty [complicated](https://www.google.com/patents/US8769944); I don't claim
to understand the details.)

In a few places you talk about confidence levels, but it's not obvious to me
if you really mean confidence level or if you mean the significance level,
typically denoted $\alpha$.

The graphs in the paper are very small and hard to read. It'd be nice if they
were larger.

Algorithm 2 doesn't really help explain what is going on beyond the 5
comments. It might be better to just list the five steps:

1. Actuator attack vector estimation;
2. State prediction;
3. State estimation;
4. Sensor attack vector estimation; and
5. Likelihood of the mode.

\subsection{Description of Change}

This submission has made major changes toward the following aspects comparing with previous submissions:
\begin{itemize}
    \item The presentation of the solution design is improved. More graphic description and plain English description on the intuition are included, and some complicated equations are moved to appendix.
    \item More explanation on why the solution works.
    \item More explanation on the evaluation results.
    \item Discuss more issues about the solution, including mode set selection, mimicry attacks, application to other robotic system, etc.
\end{itemize}
